# Supplementary material for: Hybrid Batch Attacks: Finding Black-box Adversarial Examples with Limited Queries
Source: arXiv:1908.07000 source file (2019-12-02)
Supplement: Supplementary file 1 [file 08_Appendix.tex]

%\appendix 
%\appendixpage
% new table 11




% \begin{table*}[!b]
% \centering
% \begingroup
% \setlength{\tabcolsep}{5pt} % Default value: 6pt
% \renewcommand{\arraystretch}{0.9}
% \scalebox{0.9}{
% \begin{tabular}{|c|c|c|c|c|c|c|c|c|} 
% \hline
% Metrics & \multicolumn{2}{c|}{Hybrid Success Rate (\%)} & \multicolumn{2}{c|}{Cost Reduction (\%)} & \multicolumn{2}{c|}{Fraction Worse (\%)} & \multicolumn{2}{c|}{Direct Transfer Rate (\%)} \\ 
% \hline
% \diagbox{Target Model}{Local Models} & \begin{tabular}[c]{@{}c@{}}NA-NC\end{tabular} & \begin{tabular}[c]{@{}c@{}}R-DenseN\\R-ResN\end{tabular} & \begin{tabular}[c]{@{}c@{}}NA-NC\end{tabular} & \begin{tabular}[c]{@{}c@{}}R-DenseN\\R-ResN\end{tabular} & \begin{tabular}[c]{@{}c@{}}NA-NC\end{tabular} & \begin{tabular}[c]{@{}c@{}}R-DenseN\\R-ResN\end{tabular} & \begin{tabular}[c]{@{}c@{}}NA-NC\end{tabular} & \begin{tabular}[c]{@{}c@{}}R-DenseN\\R-ResN\end{tabular} \\ 
% \hline
% Std-Dense & \textbf{99.9} & 99.3 & \textbf{68.4} & 31.4 & \textbf{4.2} & 19.6 & \textbf{63.3} & 17.0 \\ 
% \hline
% Madry Robust & 38.0 & \textbf{45.2} & 0.7 & \textbf{32.1} & 15.0 & \textbf{2.9} & 10.1 & \textbf{40.8} \\
% \hline
% \end{tabular}
% }
% \endgroup
% \caption{Performance Comparison of All Normal and All Robust Local Ensembles on Robust CIFAR10 Target Model (Attack: NES). Attack on Madry robust model is averaged over 5 independent runs: \footnotesize{\textbf{Success Rate (\%):} Robust Locals $(45.2 \pm{0.4})$, Normal Locals ($38.0 \pm{0.2}$); \textbf{Cost Reduction (\%):} Robust Locals (32.1 $\pm{1.3}$), Normal Locals ($0.7 \pm{1.3}$); \textbf{Fraction Worse (\%):} Robust Locals ($2.9 \pm{0.3}$), Normal Locals ($15.0 \pm{0.4}$); \textbf{Direct Transfers (\%):} Robust Locals ($40.8 \pm{0.3}$), Normal Locals ($10.1 \pm{0.4}$).}}
% \label{tab:nes_cifar10_local_model_comp}
% \end{table*}


% \section{More results}
% \label{appex_sec:loc_ensemble}
% In Table \ref{tab:cifar10_local_mixture}, we provide complete results of different local ensembles to both normal and robust CIFAR10 target models. 

%In Table \ref{tab:cifar10_local_mixture}, {\em Overall Transfer Rate} denotes the fraction of direct transfer of all local AEs, regardless of success to the local models. {\em Candidate Transfer Rate} denotes the fraction of direct transfer of local AEs that succeed against all local models. {\em Candidate Rate} denotes the fraction of local AEs that succeed against all local models. We measure the candidate transfer rate because, for seeds fail to attack the local models, they may have much lower likelihood to transfer to the target model and are of limited value for the attacker to consider their transferability. Results in Table \ref{tab:cifar10_local_mixture} confirm our hypothesis. Candidate transfer rate can be helpful for batch attacks in Section \ref{sec:batch_attack}, where attacker can save query by only checking transfer rates of locally successful adversarial examples when resources are limited. In Section \ref{sec:candi_sel}, we introduce more sophisticated ways of selecting candidates, where seeds can be prioritized and higher ranked seeds are better candidates.


% \begin{table*}[tbh]
% \centering
% \small
% \scalebox{0.85}{
% \begin{tabular}{|c|c|c|c|c|c|c|c|c|c|} 
% \hline
% Target Model & Metrics & R-DenseN & R-ResN & NA & NB & NC & \begin{tabular}[c]{@{}c@{}}R-DenseN\\ R-ResN\end{tabular} & \begin{tabular}[c]{@{}c@{}}R-ResN \\NA\end{tabular} & \begin{tabular}[c]{@{}c@{}}R-ResN \\NC\end{tabular} \\ 
% \hline
% \multirow{3}{*}{$\text{Std-DenseNet}$ } & Overall Transfer Rate & 14.9\% & 10.3\% & 11.2\% & 27.6\% & 53.2\% & 17.0\% & 11.2\% & 52.8\% \\ 
% \cline{2-10}
%  & Candidate Transfer Rate & 29.97\% & 23.31\% & 12.4\% & 27.6\% & 53.2\% & 43.23 & 57.14\% & 90.0\% \\ 
% \cline{2-10}
%  & Candidate Rate & 34.7\% & 32.6\% & 90.3\% & 100\% & 100\% & 19.2\% & 2.1\% & 1.0\% \\ 
% \hline
% \multirow{3}{*}{$\text{Adv-ResNet-W}$ } & Overall Transfer Rate & 33.6\% & 36.7\% & 13.0\% & 7.2\% & 5.3\% & 40.8\% & 12.9\% & 5.3\% \\ 
% \cline{2-10}
%  & Candidate Transfer Rate & 45.58\% & 48.91\% & 13.05\% & 7.2\% & 5.3\% & 62.85\% & 35.09\% & 21.54\% \\ 
% \cline{2-10}
%  & Candidate Rate & 72.4\% & 73.6\% & 99.6\% & 100\% & 100\% & 60.3\% & 32.2\% & 19.5\% \\ 
% \hline
% \multicolumn{1}{|l}{} & \multicolumn{1}{c}{} & \multicolumn{1}{c}{} & \multicolumn{1}{c}{} & \multicolumn{1}{c}{} & \multicolumn{1}{c}{} & \multicolumn{1}{c}{} & \multicolumn{1}{c}{} & \multicolumn{1}{c}{} &  \\ 
% \hline
% Target Model & Metrics & \begin{tabular}[c]{@{}c@{}}NB\\ NC \end{tabular} & \begin{tabular}[c]{@{}c@{}}R-DenseN\\NA\end{tabular} & \begin{tabular}[c]{@{}c@{}}R-DenseN\\NB\end{tabular} & \begin{tabular}[c]{@{}c@{}}R-DenseN\\NC\end{tabular} & \begin{tabular}[c]{@{}c@{}}R-ResN\\NB\end{tabular} & \begin{tabular}[c]{@{}c@{}}NA\\NB\end{tabular} & \begin{tabular}[c]{@{}c@{}}NA\\NC\end{tabular} & \begin{tabular}[c]{@{}c@{}}R-DenseN\\ANesN\\NA\end{tabular} \\ 
% \hline
% \multirow{3}{*}{$\text{Std-DenseNet}$ } & Overall Transfer Rate & 59.0\% & 11.10\% & 26.9\% & 52.9\% & 26.10\% & 36.00\% & 56.3\% & 11.5\% \\ 
% \cline{2-10}
%  & Candidate Transfer Rate & 59.06\% & 46.15\% & 71.43\% & 90.91\% & 71.43\% & 46.3\% & 65.23\% & 55.56\% \\ 
% \cline{2-10}
%  & Candidate Rate & 99.9\% & 2.6\% & 0.7\% & 1.1\% & 1.4\% & 59.4\% & 55.8\% & 0.9\% \\ 
% \hline
% \multirow{3}{*}{$\text{Adv-ResNet-W}$ } & Overall Transfer Rate & 7.3\% & 12.90\% & 7.2\% & 5.3\% & 7.10\% & 11.30\% & 9.9\% & 12.9\% \\ 
% \cline{2-10}
%  & Candidate Transfer Rate & 7.3\% & 37.15\% & 29.31\% & 23.72\% & 26.64\% & 12.74\% & 11.33\% & 43.63\% \\ 
% \cline{2-10}
%  & Candidate Rate & 100\% & 25.3\% & 17.4\% & 15.6\% & 21.4\% & 87.1\% & 86.5\% & 20.4\% \\ 
% \hline
% \multicolumn{1}{l}{} & \multicolumn{1}{l}{} & \multicolumn{1}{l}{} & \multicolumn{1}{l}{} & \multicolumn{1}{l}{} & \multicolumn{1}{l}{} & \multicolumn{1}{l}{} & \multicolumn{1}{l}{} & \multicolumn{1}{l}{} & \multicolumn{1}{l}{} \\ 
% \hline
% Target Model & Metrics & \begin{tabular}[c]{@{}c@{}}R-DenseN\\R-ResN\\NB\end{tabular} & \begin{tabular}[c]{@{}c@{}}R-DenseN\\R-ResN\\NC\end{tabular} & \begin{tabular}[c]{@{}c@{}}R-DenseN\\NA\\NB\end{tabular} & \begin{tabular}[c]{@{}c@{}}R-DenseN\\NA\\NC\end{tabular} & \begin{tabular}[c]{@{}c@{}}R-DenseN\\NB\\NC\end{tabular} & \begin{tabular}[c]{@{}c@{}}R-ResN\\NA\\NB\end{tabular} & \begin{tabular}[c]{@{}c@{}}R-ResN\\NA\\NC\end{tabular} & \begin{tabular}[c]{@{}c@{}}R-ResN\\NB\\NC\end{tabular} \\ 
% \hline
% \multirow{3}{*}{$\text{Std-DenseNet}$ } & Overall Transfer Rate & 26.00\% & 52.9\% & 35.9\% & 56.3\% & 59.30\% & 35.5\% & 56.20\% & 59.2\% \\ 
% \cline{2-10}
%  & Candidate Transfer Rate & 80\% & 75\% & 73.68\% & 100\% & 100\% & 94.44\% & 100\% & 100\% \\ 
% \cline{2-10}
%  & Candidate Rate & 0.5\% & 0.4\% & 1.9\% & 2\% & 1.1\% & 1.8\% & 1.8\% & 1.5\% \\ 
% \hline
% \multirow{3}{*}{$\text{Adv-ResNet-W}$ } & Overall Transfer Rate & 7.10\% & 5.3\% & 11.3\% & 9.9\% & 7.30\% & 11.4\% & 9.90\% & 7.3\% \\ 
% \cline{2-10}
%  & Candidate Transfer Rate & 35.34\% & 30.17\% & 36.04\% & 33.02\% & 29.51\% & 32.17\% & 31.68\% & 26.7\% \\ 
% \cline{2-10}
%  & Candidate Rate & 13.3\% & 11.6\% & 22.2\% & 21.2\% & 18.3\% & 28.6\% & 26.2\% & 22.1\% \\ 
% \hline
% \multicolumn{1}{l}{} & \multicolumn{1}{l}{} & \multicolumn{1}{l}{} & \multicolumn{1}{l}{} & \multicolumn{1}{l}{} & \multicolumn{1}{l}{} & \multicolumn{1}{l}{} & \multicolumn{1}{l}{} & \multicolumn{1}{l}{} & \multicolumn{1}{l}{} \\ 
% \hline
% Target Model & Metrics & \begin{tabular}[c]{@{}c@{}}NA\\NB\\NC\end{tabular} & \begin{tabular}[c]{@{}c@{}}R-DenseN\\R-ResN\\NA\\NB\end{tabular} & \begin{tabular}[c]{@{}c@{}}R-DenseN\\R-ResN\\NA\\NC\end{tabular} & \begin{tabular}[c]{@{}c@{}}R-DenseN\\R-ResN\\NB\\NC\end{tabular} & \begin{tabular}[c]{@{}c@{}}R-DenseN\\NA\\NB\\NC\end{tabular} & \begin{tabular}[c]{@{}c@{}}R-ResN\\NA\\NB\\NC\end{tabular} & \multicolumn{2}{c|}{\begin{tabular}[c]{@{}c@{}} R-DenseN R-ResN\\NA NB\\NC\end{tabular}} \\ 
% \hline
% \multirow{3}{*}{$\text{Std-DenseNet}$ } & Overall Transfer Rate & 63.3\% & 35.5\% & 56.20\% & 58.90\% & 63.40\% & 63.3\% & \multicolumn{2}{c|}{63.5\%} \\ 
% \cline{2-10}
%  & Candidate Transfer Rate & 75.66\% & 88.89\% & 100\% & 100\% & 89.47\% & 100\% & \multicolumn{2}{c|}{88.89\%} \\ 
% \cline{2-10}
%  & Candidate Rate & 41.9\% & 0.9\% & 0.7\% & 0.6\% & 1.9\% & 1.8\% & \multicolumn{2}{c|}{0.9\%} \\ 
% \hline
% \multirow{3}{*}{ $\text{Adv-ResNet-W}$ } & Overall Transfer Rate & 10.1\% & 11.3\% & 10.00\% & 7.30\% & 9.50\% & 9.5\% & \multicolumn{2}{c|}{ 9.5\%} \\ 
% \cline{2-10}
%  & Candidate Transfer Rate & 11.89\% & 39.78\% & 42.5\% & 36.3\% & 33.49\% & 28.63\% & \multicolumn{2}{c|}{ 39.05\%} \\ 
% \cline{2-10}
%  & Candidate Rate & 75.7\% & 18.1\% & 16\% & 13.5\% & 21.2\% & 26.2\% & \multicolumn{2}{c|}{16.90\%} \\
% \hline
% \end{tabular}
% }
% \caption{Direct transfer rates of different local ensembles to CIFAR10 target models: \footnotesize{{\em Overall Transfer Rate} denotes the fraction of direct transfer of all local AEs, regardless of success to the local models. {\em Candidate Transfer Rate} denotes the fraction of direct transfer of local AEs that succeed against all local models. {\em Candidate Rate} denotes the fraction of local AEs that succeed against all local models. Third to last columns denote different local ensembles. R-DenseN denotes adversarially trained DenseNet model, R-ResN denotes adversarially trained ResNet model. NA, NB and NC are normal local models.}}
% \label{tab:cifar10_local_mixture}
% \end{table*}





%\subsection{Candidate Selection and Candidate Transfer rate}
%The problem with blindly treating all locally generated AEs as candidates (as is in Section \ref{sec:improve_robust_attack}) is problematic as some seeds fail to attack the local models and therefore, have much lower likelihood to transfer to the target model and of limited value for the attacker to consider transferability of the failed AEs. We validate the statement by checking the candidate transfer rate and non-candidate transfer rates individually, where candidates are chosen as AEs that succeed against all the local models. In general, candidate transfer rate is much higher than the non-candidate transfer rate and the overall transfer rate. More details regarding candidate rate and candidate transfer rate can be found in Table \ref{tab:cifar10_local_mixture}. For example, the targeted candidate transfer rate from Adv-DenseNet to standard CIFAR10 DenseNet model (column of R-DenseN in Table \ref{tab:cifar10_local_mixture}) is 29.97\% while targeted non-candidate transfer rate is only 6.9\% (more than 4 times improvement), and the overall transfer rate is 14.9\% (2 times improvement). Another example is the untargeted transfer rate from ensemble of (R-ResN,NC) to Madry CIFAR10 robust model, the candidate transfer rate is 21.54\% while the non-candidate transfer rate is only 1.37\%, and the overall transfer rate is only 5.3\%. In addition, if we consider from the perspective of candidate transfer rate, we can find universal local ensemble with reasonably high candidate transfer rate to both normal and robust target models. One example is the local ensemble of (R-DenseN,R-ResN) in Table \ref{tab:cifar10_local_mixture} with candidate transfer rate of 43.23\% (candidate rate of 19.2\%) and 62.85\% (candidate rate of 60.3\%) to normal and robust target model respectively.

%Candidate selection criteria can be helpful for batch attacks, where the query resource is limited. By carefully selecting the candidates, attacker can obtain much more number of AEs by querying only the candidates within the limited query budget as majority of the candidates may directly transfer. We provide detailed discussion on this in Section \ref{sec:first_stage_eval}. For CIFAR10 models, since there are 31 different local ensembles, in later sections, we only choose local ensembles of all normal and all robust models as these two give higher transfer rate to normal target and robust target models respectively.

%By considering locally successful AEs as candidates, we also present several interesting findings below (however, these surprising findings can be explained by the different attack surfaces of normal and robust models (Section \ref{sec:improve_robust_attack})):
% \begin{itemize} 
%     \item When one normal and one robust models are mixed, the candidate rate drops compared to the case of two normal or two robust models (see columns of (R-DenseN,R-ResN), (R-ResN,NA), (R-ResN,NC) and (NB,NC) in Table \ref{tab:cifar10_local_mixture}). Normal models are easier to be attacked and therefore, when mixed with a robust model, expected candidate rate should be higher than the ensembles of two robust models. The observation is quite surprising and it can be explained by the differences of normal and robust models: different attack surfaces of the two models make the attack harder to find a reliable perturbation for both as the blind spots of robust and normal models are different.   
%     \item Addition of normal local models to robust local models reduces the candidate rate (as expected), but in the meantime, the candidate transfer rate is also reduced, compared to the case of all robust local models (see ensembles of (R-DenseN,R-ResN),(R-DenseN,R-ResN,NA) and (R-DenseN,R-ResN,NA,NB) in Table \ref{tab:cifar10_local_mixture}). With addition of more local models, expected result is the drop in candidate rate and the increase in candidate transfer rate as the candidate selection criteria becomes stricter. One possible reason for this finding is, different attack surfaces of normal and robust models generates candidate AEs with lower quality and therefore, leads to decreased candidate transfer rate, although candidate selection criteria is stricter. 
%     \item Individual model with higher transfer rate to robust target model of lower transfer rate to normal target model (see the first five columns of individual models in Table \ref{tab:cifar10_local_mixture}). This also demonstrates the different attack surfaces of normal and robust models. Note that, among the three normal local models, NC with the most complex structure has lowest transferability to robust target model while NA with simplest structure has highest transferability. Currently, we are unclear why a simple normal model transfer better to robust target model to relatively more complex normal models (i.e., NB, NC). It is interesting to check if there is a connection between complexity of normal models and their transferability to robust models.
% \end{itemize}


% \begin{table}[tb]
% \centering
% \scriptsize
% \scalebox{0.9}{
% \begin{tabular}{|c|c|c|c|c|c|c|}
% \hline
% \multicolumn{3}{|c|}{AutoZOOM} &  & \multicolumn{3}{c|}{NES} \\ \cline{1-3} \cline{5-7} 
%  & \begin{tabular}[c]{@{}c@{}}NA\\ NB\\ NC \end{tabular} & \begin{tabular}[c]{@{}c@{}}R-DenseN\\ R-ResN\end{tabular} &  &  & \begin{tabular}[c]{@{}c@{}}NA\\ NB\\ NC\end{tabular} & \begin{tabular}[c]{@{}c@{}}R-DenseN\\ R-ResN\end{tabular} \\ \cline{1-3} \cline{5-7} 
% \begin{tabular}[c]{@{}c@{}}$\text{Std-Dense}^{+}$\end{tabular} & 98.1\% & 95.6\% &  & \begin{tabular}[c]{@{}c@{}}$\text{Std-Dense}^{+}$\end{tabular} & 99.9\% & 99.3\% \\ \cline{1-3} \cline{5-7} 
% $\text{Adv-ResNet-W}^{-}$ & 65.2\% & 68.7\% &  & $\text{Adv-ResNet-W}^{-}$ & 31.1\% & 43.2\% \\ \hline
% \end{tabular}
% }
% \caption{Hybrid success rate of normal and robust local ensembles on CIFAR10 target models: \footnotesize{``+'' means targeted attack on the target model. ``-'' means untargeted attack on the target model. Each cell $(i,j)$ denotes the pair of target model $i$ and local ensemble $j$. ADesne means the adversarially trained DenseNet Model. R-ResN mneas the adversarially trained ResNet model. For normal target model, baseline success rates of AutoZOOM and NES attack are 92.2\% and 99.1\% respectively. For robust target model, baseline success rates of AutoZOOM and NES are 65.2\% and 31.1\% respectively.}}
% \label{tab:cifar10_hybrid_succ_rate}
% \end{table}

% \begin{table}[tb]
% \scriptsize
% \scalebox{0.9}{
% \begin{tabular}{|c|c|c|c|c|c|c|}
% \hline
% \multicolumn{3}{|c|}{AutoZOOM} &  & \multicolumn{3}{c|}{NES} \\ \cline{1-3} \cline{5-7} 
%  & \begin{tabular}[c]{@{}c@{}}NA\\ NB\\ NC\end{tabular} & \begin{tabular}[c]{@{}c@{}}R-DenseN\\ R-ResN\end{tabular} &  &  & \begin{tabular}[c]{@{}c@{}}NA\\ NB\\ NC\end{tabular} & \begin{tabular}[c]{@{}c@{}}R-DenseN\\ R-ResN\end{tabular} \\ \cline{1-3} \cline{5-7} 
% \begin{tabular}[c]{@{}c@{}}$\text{Std-Dense}^{+}$\end{tabular} & 77.3\% & 68.0\% &  & \begin{tabular}[c]{@{}c@{}}$\text{Std-Dense}^{+}$\end{tabular} & 68.4\% & 31.4\% \\ \cline{1-3} \cline{5-7} 
% $\text{Adv-ResNet-W}^{-}$ & 4.1\% & 21.0\% &  & $\text{Adv-ResNet-W}^{-}$ & 0.4\% & 45.8\% \\ \hline
% \end{tabular}
% }
% \caption{Mean cost reduction in queries of normal and robust local ensembles on CIFAR10 target models: \footnotesize{``+'' means targeted attack on the target model. ``-'' means untargeted attack on the target model. For normal target model, baseline mean query of AutoZOOM and NES attack are 1,223 and 1,098 respectively. For robust target model, baseline mean query of AutoZOOM and NES are 2,638 and 9,887 respectively.}}
% \label{tab:cifar10_mean_cost_reduction}
% \end{table}

% \begin{table}[t]
% \scriptsize
% \scalebox{0.9}{
% \begin{tabular}{|c|c|c|c|c|c|c|}
% \hline
% \multicolumn{3}{|c|}{AutoZOOM} &  & \multicolumn{3}{c|}{NES} \\ \cline{1-3} \cline{5-7} 
%  & \begin{tabular}[c]{@{}c@{}}NA\\ NB\\ NC\end{tabular} & \begin{tabular}[c]{@{}c@{}}R-DenseN\\ R-ResN\end{tabular} &  &  & \begin{tabular}[c]{@{}c@{}}NA\\ NB\\ NC\end{tabular} & \begin{tabular}[c]{@{}c@{}}R-DenseN\\ R-ResN\end{tabular} \\ \cline{1-3} \cline{5-7} 
% \begin{tabular}[c]{@{}c@{}}$\text{Std-Dense}^{+}$\end{tabular} & 0.013 & 0.126 &  & \begin{tabular}[c]{@{}c@{}}$\text{Std-Dense}^{+}$\end{tabular} & 0.042 & 0.196 \\ \cline{1-3} \cline{5-7} 
% $\text{Adv-ResNet-W}^{-}$ & 0.256 & 0.044 &  & $\text{Adv-ResNet-W}^{-}$ & 0.138 & 0.017 \\ \hline
% \end{tabular}
% }
% \caption{Worse fraction of normal and robust local ensembles on CIFAR10 target models: \footnotesize{``+'' means targeted attack on the target model. ``-'' means untargeted attack on the target model.}}
% \label{tab:cifar10_worse_fraction}
% \end{table}




    
